# Supplementary material for: Timing and spectral variability of high mass X-ray pulsar GX 301--2 over orbital phases observed by Insight-HXMT
Source: arXiv:2106.14603 source file (2021-06-28)
Supplement: Supplementary file 1 [file supplementary.pdf]

## **Supplementary Material**

Tab. 1: Log of GX 301–2 observations

| OBSID         | Start Date | Start MJD | Orbital Phase |
|---------------|------------|-----------|---------------|
| P010130900101 | 2017-08-03 | 57968.24  | 0.952         |
| P010130900102 | 2017-08-03 | 57968.41  | 0.956         |
| P010130900103 | 2017-08-03 | 57968.54  | 0.959         |
| P010130900104 | 2017-08-03 | 57968.68  | 0.963         |
| P010130900105 | 2017-08-03 | 57968.81  | 0.966         |
| P010130900106 | 2017-08-03 | 57968.94  | 0.969         |
| P010130900107 | 2017-08-04 | 57969.07  | 0.972         |
| P010130900401 | 2017-08-04 | 57969.50  | 0.983         |
| P010130900402 | 2017-08-04 | 57969.67  | 0.987         |
| P010130900403 | 2017-08-04 | 57969.81  | 0.990         |
| P010130900404 | 2017-08-04 | 57969.94  | 0.993         |
| P010130900501 | 2018-01-03 | 58121.11  | 0.637         |
| P010130900502 | 2018-01-03 | 58121.24  | 0.641         |
| P010130900503 | 2018-01-03 | 58121.38  | 0.644         |
| P010130900601 | 2018-01-04 | 58122.24  | 0.665         |
| P010130900602 | 2018-01-04 | 58122.38  | 0.668         |
| P010130900701 | 2018-01-19 | 58137.47  | 0.032         |
| P010130900702 | 2018-01-19 | 58137.65  | 0.036         |
| P010130900703 | 2018-01-19 | 58137.80  | 0.040         |
| P010130900704 | 2018-01-19 | 58137.93  | 0.043         |
| P010130900705 | 2018-01-20 | 58138.04  | 0.046         |
| P010130900706 | 2018-01-20 | 58138.18  | 0.049         |
| P010130900707 | 2018-01-20 | 58138.31  | 0.052         |
| P010130900708 | 2018-01-20 | 58138.44  | 0.055         |
| P010130900709 | 2018-01-20 | 58138.58  | 0.058         |
| P010130900710 | 2018-01-20 | 58138.73  | 0.062         |
| P010130900711 | 2018-01-20 | 58138.86  | 0.065         |
| P010130900801 | 2018-01-29 | 58147.41  | 0.271         |
| P010130900802 | 2018-01-29 | 58147.60  | 0.276         |
| P010130900803 | 2018-01-29 | 58147.74  | 0.279         |
| P010130900804 | 2018-01-29 | 58147.87  | 0.283         |
| P010130900805 | 2018-01-29 | 58148.01  | 0.286         |
| P010130900806 | 2018-01-30 | 58148.14  | 0.289         |
| P010130900807 | 2018-01-30 | 58148.53  | 0.298         |
| P010130900808 | 2018-01-30 | 58148.66  | 0.302         |
| P010130900809 | 2018-01-30 | 58148.80  | 0.305         |
| P010130900901 | 2018-02-13 | 58162.93  | 0.646         |
| P010130900902 | 2018-02-14 | 58163.13  | 0.650         |
| P010130900903 | 2018-02-14 | 58163.26  | 0.654         |
| P010130901001 | 2018-03-02 | 58179.43  | 0.043         |
| P010130901003 | 2018-03-02 | 58179.76  | 0.051         |
| P010130901101 | 2018-03-04 | 58181.62  | 0.096         |
| P010130901201 | 2018-03-05 | 58182.41  | 0.115         |
| P010130901301 | 2018-03-06 | 58183.61  | 0.144         |
| P010130901401 | 2018-03-07 | 58184.47  | 0.165         |
| P010130901501 | 2018-04-09 | 58217.83  | 0.969         |
| P010130901601 | 2018-05-20 | 58258.27  | 0.944         |
| P010130901602 | 2018-05-20 | 58258.44  | 0.948         |
| P010130901603 | 2018-05-20 | 58258.57  | 0.951         |
| P010130901701 | 2018-05-21 | 58259.79  | 0.981         |
| P010130901702 | 2018-05-21 | 58259.93  | 0.984         |
| P010130901703 | 2018-05-22 | 58260.06  | 0.987         |
| P010130901801 | 2018-07-27 | 58326.85  | 0.597         |

Tab. 2: Log of GX 301–2 observations

| OBSID         | Start Date | Start MJD | Orbital Phase |
|---------------|------------|-----------|---------------|
| P010130901802 | 2018-07-27 | 58326.98  | 0.600         |
| P010130902001 | 2019-01-12 | 58495.69  | 0.667         |
| P010130902101 | 2019-03-03 | 58545.28  | 0.863         |
| P010130902102 | 2019-03-03 | 58545.45  | 0.867         |
| P010130902103 | 2019-03-03 | 58545.58  | 0.870         |
| P010130902104 | 2019-03-03 | 58545.72  | 0.873         |
| P020101228001 | 2019-07-06 | 58670.35  | 0.899         |
| P020101228002 | 2019-07-06 | 58670.48  | 0.899         |
| P020101228003 | 2019-07-06 | 58670.62  | 0.923         |
| P020101228004 | 2019-07-06 | 58670.75  | 0.923         |
| P020101228005 | 2019-07-06 | 58670.88  | 0.923         |
| P020101228006 | 2019-07-07 | 58671.01  | 0.923         |
| P020101228007 | 2019-07-07 | 58671.15  | 0.923         |
| P020101228101 | 2019-07-16 | 58680.62  | 0.164         |
| P020101228103 | 2019-07-17 | 58681.09  | 0.164         |
| P020101228104 | 2019-07-17 | 58681.23  | 0.164         |
| P020101228105 | 2019-07-17 | 58681.37  | 0.164         |
| P020101228106 | 2019-07-17 | 58681.51  | 0.189         |
| P020101228201 | 2019-08-12 | 58707.07  | 0.791         |
| P020101228202 | 2019-08-12 | 58707.22  | 0.791         |
| P020101228203 | 2019-08-12 | 58707.35  | 0.791         |
| P020101228204 | 2019-08-12 | 58707.48  | 0.791         |
| P020101228205 | 2019-08-12 | 58707.61  | 0.816         |
| P020101228207 | 2019-08-12 | 58707.88  | 0.816         |
| P020101228301 | 2020-01-12 | 58860.27  | 0.481         |
| P020101228302 | 2020-01-12 | 58860.41  | 0.481         |
| P020101228303 | 2020-01-12 | 58860.56  | 0.505         |
| P020101228304 | 2020-01-12 | 58860.69  | 0.505         |
| P020101228305 | 2020-01-12 | 58860.83  | 0.505         |
| P020101228306 | 2020-01-12 | 58860.96  | 0.505         |
| P020101228401 | 2020-01-15 | 58863.58  | 0.577         |
| P020101228402 | 2020-01-15 | 58863.74  | 0.577         |
| P020101228403 | 2020-01-15 | 58863.87  | 0.577         |
| P020101228404 | 2020-01-16 | 58864.0   | 0.577         |
| P020101228405 | 2020-01-16 | 58864.14  | 0.577         |
| P020101228406 | 2020-01-16 | 58864.27  | 0.577         |
| P020101228407 | 2020-01-16 | 58864.4   | 0.577         |
| P020101228501 | 2020-01-20 | 58868.08  | 0.674         |
| P020101228502 | 2020-01-20 | 58868.22  | 0.674         |
| P020101228503 | 2020-01-20 | 58868.38  | 0.674         |
| P020101228504 | 2020-01-20 | 58868.51  | 0.698         |
| P020101228505 | 2020-01-20 | 58868.64  | 0.698         |
| P020101228506 | 2020-01-20 | 58868.78  | 0.698         |
| P020101228507 | 2020-01-20 | 58868.91  | 0.698         |
| P020101228603 | 2020-01-29 | 58877.60  | 0.915         |
| P020101228605 | 2020-01-29 | 58877.88  | 0.915         |
| P020101228606 | 2020-01-30 | 58878.02  | 0.915         |
| P020101228608 | 2020-01-30 | 58878.52  | 0.939         |
| P020101228610 | 2020-01-30 | 58878.80  | 0.939         |
| P020101228611 | 2020-01-30 | 58878.94  | 0.939         |
| P020101228701 | 2020-02-14 | 58893.53  | 0.300         |
| P020101228702 | 2020-02-14 | 58893.71  | 0.300         |
| P020101228703 | 2020-02-14 | 58893.85  | 0.300         |

Tab. 3: Log of GX 301–2 observations

| OBSID         | Start Date | Start MJD | Orbital Phase |
|---------------|------------|-----------|---------------|
| P020101228704 | 2020-02-14 | 58893.98  | 0.300         |
| P020101228705 | 2020-02-15 | 58894.11  | 0.300         |
| P020101228706 | 2020-02-15 | 58894.24  | 0.300         |
| P020101228707 | 2020-02-15 | 58894.38  | 0.300         |
| P020101228801 | 2020-03-18 | 58926.41  | 0.072         |
| P020101228802 | 2020-03-18 | 58926.57  | 0.096         |
| P020101228803 | 2020-03-18 | 58926.70  | 0.096         |
| P020101228804 | 2020-03-18 | 58926.83  | 0.096         |
| P020101228805 | 2020-03-18 | 58926.96  | 0.096         |
| P020101228806 | 2020-03-19 | 58927.10  | 0.096         |
| P020101228807 | 2020-03-19 | 58927.23  | 0.096         |
| P020101228901 | 2020-04-06 | 58945.10  | 0.530         |
| P020101228902 | 2020-04-06 | 58945.25  | 0.530         |
| P020101228903 | 2020-04-06 | 58945.39  | 0.530         |
| P020101228904 | 2020-04-06 | 58945.53  | 0.554         |
| P020101228905 | 2020-04-06 | 58945.67  | 0.554         |
| P020101228906 | 2020-04-06 | 58945.81  | 0.554         |
| P020101229001 | 2020-06-03 | 59003.30  | 0.929         |
| P020101229002 | 2020-06-03 | 59003.45  | 0.929         |
| P020101229003 | 2020-06-03 | 59003.59  | 0.953         |
| P020101229004 | 2020-06-03 | 59003.73  | 0.953         |
| P020101229101 | 2020-06-04 | 59004.42  | 0.953         |
| P020101229102 | 2020-06-04 | 59004.59  | 0.977         |
| P020101229103 | 2020-06-04 | 59004.73  | 0.977         |
